# Supplementary material for: Monopole density and antiferromagnetic domain control in spin-ice iridates
Source: arXiv:2102.04483 source file (2021-02-08)
Supplement: Supplementary file 2 [file reftest4-2.tex]

% ****** Start of file reftest.tex ******
%
%   This file is part of the APS files in the REVTeX 4.2 distribution.
%   Version 4.2a of REVTeX, December, 2014.
%
%   Copyright (c) 2014 The American Physical Society.
%
%   See the REVTeX 4.2 README file for restrictions and more information.
%
\documentclass{revtex4}%
\begin{document}%

\typeout{Filename: reftest4-2.tex for revtex 4.X 2014/12/31 (AO)}
% This document, when typeset, prompts for the name of a LaTeX auxiliary (.aux) file 
% and then processes that file, paying attention to 
% keys that have been cited (via \citation)
% or defined (via \bibcite).
% It then prints out diagnostics indicating 
% * any keys that were cited but never defined,
% * any keys that were defined but never cited, and
% * keys that were cited and defined, but not in the same order.
%
% BibTeX takes care of such things automatically,
% so there is little use for such a test when using BibTeX.
%
% A separate question: will this file run under revtex4.cls?
% I can see two lines in my .aux with the potential for problems: 
% \global \mathchardef \firstnote@num\z@ \relax 
% \global\NAT@numberstrue

\makeatletter

\def\g@bbletw@#1#2{}%
\def\g@bble@ne#1{}%

\let\bibdata\g@bble@ne
\let\newlabel\g@bbletw@
\let\@writefile\g@bbletw@
\let\bibstyle\g@bble@ne

\@tempcnta\z@
\@tempcntb\z@

\def\bibcite#1#2{%
 \advance\@tempcnta\@ne
 \expandafter\bib@one\csname bib#1\expandafter\endcsname\expandafter{\the\@tempcnta}{#1}%
}

\def\bib@one#1#2#3{%
 \@ifnotrelax#1{%
  \typeout{*** Tag "#3" used in more than one \string\bibitem.}%
  \typeout{\space\space\space\space You must correct this problem before continuing (Bailing out).}%
  \@@end
 }{%
  \def#1{#2}%
  \expandafter\def\csname bib@num#2\endcsname{#3}%
 }%
}%

\def\citation#1{%
 \@for\@tempa:={#1}\do{%
  \expandafter\cite@one\csname cite\@tempa\expandafter\endcsname\expandafter{\@tempa}%
 }%
}

\def\cite@one#1#2{%
 \expandafter\@ifx\expandafter{\csname cite*\endcsname#1}{%
  \@booleantrue\@cite@star@sw
 }{%
  \@ifnotrelax#1{%
  }{%
   \advance\@tempcntb\@ne
   \expandafter\cite@one@\expandafter#1\expandafter{\the\@tempcntb}{#2}%
  }%
 }%
}%
\expandafter\def\csname cite*\endcsname{*}%
\@booleanfalse\@cite@star@sw

\def\cite@one@#1#2#3{%
 \def#1{#2}%
 \expandafter\def\csname cite@num#2\endcsname{#3}%
}%

\def\strut{\vrule height12pt depth4pt width0pt}%

\typein[\filename]{Type in file name (no extension)}%
\expandafter\input\expandafter{\filename.aux}%

\expandafter\def\expandafter\bibtotal\expandafter{\the\@tempcnta}%
\expandafter\def\expandafter\citetotal\expandafter{\the\@tempcntb}%

\def\app@undefined#1#2#3{%
 \expandafter\@ifnotrelax\csname#2#1\endcsname{}{%
   \appdef#3{#1, }%
  }
}%

\let\uncitedbibs\@empty
\@tempcnta\z@
\@ifnum{\bibtotal>\@tempcnta}{%
 \loopwhile{%
  \advance\@tempcnta\@ne
  \expandafter\app@undefined\csname bib@num\the\@tempcnta\endcsname{cite}\uncitedbibs
  \@ifnum{\bibtotal>\@tempcnta}%
 }%
}%

\let\undefinedcites\@empty
\@tempcnta\z@
\@ifnum{\citetotal>\@tempcnta}{%
 \loopwhile{%
  \advance\@tempcnta\@ne
  \expandafter\app@undefined\csname cite@num\the\@tempcnta\endcsname{bib}\undefinedcites
  \@ifnum{\citetotal>\@tempcnta}%
 }%
}%

\def\addit@bad#1#2{%
 \expandafter\@ifnotrelax\csname bib#1\endcsname{%
  \@ifx{#1#2}{%
   \addit{#1}{OK}%
  }{%
   \advance\@tempcntb\@ne
   \addit{#1}{\bf Out of order}%
  }%
 }{%
  \addit{#1}{\bf Undefined}%
 }%
}%
\def\ordertable{}%
\def\table@line#1#2{%
  \hbox to\hsize{%
   \vrule
   \hbox to.5\hsize{\ #1\hss}%
   \hss\vrule\hss\strut
   \hbox to.5\hsize{\ #2\hss}%
   \vrule
  }%
  \hrule
  \vskip\z@skip
}%
\def\addit#1#2{%
 \appdef\ordertable{\table@line{#1}{#2}}%
}%

\@tempcnta\z@
\@tempcntb\z@
\@ifnum{\citetotal>\@tempcnta}{%
 \loopwhile{%
  \advance\@tempcnta\@ne
  \expandafter\addit@bad\csname cite@num\the\@tempcnta\expandafter\endcsname\csname bib@num\the\@tempcnta\endcsname
  \@ifnum{\citetotal>\@tempcnta}%
 }%
}{}%
\expandafter\def\expandafter\citesdisordered\expandafter{\the\@tempcntb}%

Analysis of \filename.aux, according to rules of \emph{Physical Review}:
All bibitems must occur in the bibliography in order of their first citation in the
file, and all bibitems must be cited in the paper.

\def\@tempa{\textbf{Bibitems that were not explicitly cited:} }%
\@ifx@empty\uncitedbibs{%
 \appdef\@tempa{none.}%
}{%
 \appdef\@tempa{\uncitedbibs\ \@cite@star@sw{were implicitly cited.}{please cite or remove bibitem(s).}}%
}%
\@tempa\expandafter\typeout\expandafter{\@tempa}\par

\def\@tempa{\textbf{Citations not defined in bibliography:} }%
\@ifx@empty\undefinedcites{%
 \appdef\@tempa{none.}%
}{%
 \appdef\@tempa{\undefinedcites\space please add bibitem(s) or remove cite(s).}%
}%
\@tempa\expandafter\typeout\expandafter{\@tempa}\par

\@ifnum{\citesdisordered=\z@}{%
 \def\@tempa{\textbf{The order of the bibitems is OK.}}%
 \@tempa\expandafter\typeout\expandafter{\@tempa}\par
}{%
 \def\@tempa{%
  \textbf{There 
  \@ifnum{\citesdisordered<\tw@}{was an error}{were \citesdisordered\ errors}
  in the order of your bibitems.}%
 }%
 \@tempa\expandafter\typeout\expandafter{\@tempa}
 \@ifx@empty\uncitedbibs{\@ifx@empty\undefinedcites{\true@sw}{\false@sw}}{\false@sw}%
 {(This is in addition to the problems noted above.) }{}%
 Please check the following table to see what the problems were.
 Status in boldface signifies that a correction is needed. \par
}%
 \emph{NOTE:
  This table is a complete listing of all your citations, in order of their first occurrence: 
  your bibitems should be in the order shown in the first column of this table.
 }\par
 \small
 \smallskip
 \hrule
 \table@line{\textbf{Citation key}}{\textbf{Status}}%
 \smallskip
 \hrule
 \ordertable
\end{document}
